# Supplementary material for: Mini-Batch Consistent Slot Set Encoder for Scalable Set Encoding
Source: arXiv:2103.01615 source file (2021-10-26)
Supplement: Supplementary file 1 [file supplementary.tex]

\documentclass{article}

% if you need to pass options to natbib, use, e.g.:
     \PassOptionsToPackage{numbers, compress}{natbib}
% before loading neurips_2021

% ready for submission
\usepackage[final]{neurips_2021}

% to compile a preprint version, e.g., for submission to arXiv, add add the
% [preprint] option:
%     \usepackage[preprint]{neurips_2021}

% to compile a camera-ready version, add the [final] option, e.g.:
%     \usepackage[final]{neurips_2021}

% to avoid loading the natbib package, add option nonatbib:
%    \usepackage[nonatbib]{neurips_2021}

\usepackage[utf8]{inputenc} % allow utf-8 input
%\usepackage[T1]{fontenc}    % use 8-bit T1 fonts
%\usepackage{hyperref}       % hyperlinks
%\usepackage{url}            % simple URL typesetting
%\usepackage{booktabs}       % professional-quality tables
%\usepackage{amsfonts}       % blackboard math symbols
%\usepackage{nicefrac}       % compact symbols for 1/2, etc.
%\usepackage{microtype}      % microtypography
%\usepackage{xcolor}         % colors
%\usepackage{graphicx}
%\usepackage{subcaption}
%\usepackage{amsmath}
%\usepackage{wrapfig}
%\usepackage{amssymb}
%\usepackage{amsthm}
%
%\definecolor{Red}{rgb}{0.768, 0.054, 0.054}
%\definecolor{Blue}{rgb}{0.152, 0.294, 0.925}
%\definecolor{Green}{rgb}{0,0.4,0.7}
%\hypersetup{
%    colorlinks=true,
%    citecolor=Red,
%    linkcolor=Blue,
%    urlcolor=Green,
%    }
%\usepackage{algorithm}
%\usepackage{algpseudocode}
%\usepackage[font=footnotesize]{caption}
%
%
%\title{Appendix: Mini-Batch Consistent Slot Set Encoder for Scalable Set Encoding}
%
%%\author{Andreis Bruno$^{1}$, Jeffrey Ryan Willette$^{1}$, Juho Lee$^{1,2}$, Sung Ju Hwang$^{1,2}$\\
%%    KAIST $^{1}$, South Korea\\AITRICS $^{2}$, South Korea \\
%%    \texttt{\{andries, jwillette, juholee, sjhwang82\}@kaist.ac.kr}
%%}
%\newtheorem{property}{Property}
%\newtheorem{proposition}{Proposition}
%\newtheorem{definition}{Definition}
%
%\begin{document}
%\maketitle
%\appendix
%
%\vspace{-0.8in}
%
%\input{sections/appendix}
%
%\begin{small}
%\bibliographystyle{abbrvnat}
%\bibliography{bibs/bibs}
%\end{small}
%\end{document}
